# Supplementary material for: Rescaling invariance and anomalous energy transport in a small vertical column of grains
Source: arXiv:2310.19475 source file (2023-10-30)
Supplement: Supplementary file 1 [file Gnoli_et_al_arxiv_SI.pdf]

# Supplemental Material:
# Rescaling invariance and anomalous energy transport in a vertical column of grains

A. Gnoli, G. Pontuale, A. Puglisi and A. Petri

## EXPERIMENTAL SET UP AND PROCESSING

### The mechanical system

The investigated system consists of a set of $N = 10$ identical steel beads of diameter $d =$ 4 mm, confined in vertical channel digged in a PMMA cylinder (Fig. S1). The channel has a square section, of side 4.1 mm, and is covered with a PVC film to reduce friction between beads and walls. A vertical slit allows air to flux in and out, so reducing viscous damping.

The energy is supplied to the system by a rigid PMMA piston that can move along the vertical at the bottom of the channel. The piston is disconnected from the pipe, which is at rest in the laboratory frame, and is moved by an electrodynamic shaker (Bruel&Kiel©, Type 4809) powered by an electronic wave generator (Agilent 33250A) through an audio amplifier. An accelerometer (Bruel & Kjaer Type 4333) is connected to the piston and the signal is sent to an acquisition board (USB-6353 by National Instruments) and sampled at a frequency of 100 Kz. In the experiments considered here the piston is driven sinusoidally. This driving is preferred to withe noise [1–5] since there is a limited frequency band where the system can be excited and applying vibrations in a wide range is uselessly energy demanding. Experiments with different amplitudes have been conducted in order to explore regimes ranging from also collapsed to well fluidized. In each experiment amplitude is kept constant. Quantities characterizing the piston motion for the different experiments are reported in Tab. I.

### Image processing

Digital images of the beads have been acquired by a camera Casio© EX-ZR100 with a gray scale digital filter, at a rate of 480 fps and a fixed focal of 57 mm. A white plate placed on the opposite side of the tube supplies a diffuse and uniform illumination (Fig. S2 (left)). Images are then acquired by a PC (through free software such as*ffmpeg* and *mogrify*). The resulting jpeg images, typically 186x12 pixel and 8 bits, represent the beads as black spots on a light background (Fig. S2 (right)). They are then processed by a script in *Octave* language which loads each image as a matrix and returns a 1D vector representing the inverted average luminosity level for each horizontal pixel stripe, graphically represented in Fig. S3. Each maximum is fitted with a parabola whose center is assumed as the center of the of the ball at the time of the corresponding frame. The final result consists of a data series for

each bead, representing the estimated position of the center in each frame, expressed in pixels. Conversion to millimeters and seconds is done through calibration images purposely acquired.

## RECONSTRUCTION OF THE DYNAMICS

### Kinematics

Examples of reconstructed trajectories are shown in Fig. S4. The particle index $1 \leq i \leq 10$ increases from bottom up. The vertical axis reports $z_i(t)$, the distance from the average position of the head of the piston. Here and in the next figures it is expressed in pixels (px), and time as number of frames (f), with 1 px=0.46 mm and 1 f=1/480 s $\simeq$ 21 ms.

From samples of binary collisional events, like those shown in Fig. S5, we have got an estimate of the restitution coefficient defined as

$$\epsilon = \frac{\dot{z}_1' - \dot{z}_2'}{\dot{z}_2 - \dot{z}_1}, \tag{1}$$

where dots stay for time derivatives and aftershock quantities are primed. We found $\epsilon \simeq 0.92$, compatible with values reported in the literature [6, 7]. In addition we have considered the trajectories of grains between consecutive collisions, like those in Fig. S6. Parabolic functions fit very well to them, with values of the gravity acceleration around $g \simeq 0.092$ pix/f$^2$, showing that other sources of energy dissipation than inter-grain collisions, like air viscosity or wall friction, are negligible.

### Fields

Fields have been defined as time averages, that in the continuous form read

$$\rho(z) = \sum_i < \delta(z - z_i(t)) > \tag{2}$$

$$u(z) = \frac{1}{N} \sum_i < \dot{z}_i(t) \delta(z - z_i(t)) > \tag{3}$$

$$T(z) = \frac{1}{N} \sum_i < (\dot{z}_i(t) - u(z))^2 \delta(z - z_i(t)) >, \tag{4}$$

where the brackets are time averages (note that density is defined such that $\int \rho \, dz = N$). Experimentally they have been computed from the data series as

$$\begin{aligned}\rho(z) &= \frac{\sum_f \sum_i \delta_{z,z_i}}{S}\\ u(z) &= \frac{\sum_f \sum_i \dot{z}_i \delta_{z,z_i}}{S}\\ T(z) &= \frac{\sum_f \sum_i (\dot{z}_i - u(z))^2 \delta_{z,z_i}}{S},\end{aligned}$$

where $S$ is the total number of points (frames) in the series and $f$ is the frame index.

| set | $A(\pm 0.05)$ (mm) | $\Gamma$ | $v_0$ (mm/s) | $T_0$ (mm/s $^2 \cdot 10^4$) |
|---|---|---|---|---|
| S1 | 2.90 | 10.6 | 549.8 | 30.22 |
| S2 | 2.85 | 10.3 | 534.0 | 28.52 |
| S3 | 2.50 | 9.1 | 471.2 | 22.20 |
| S4 | 2.15 | 7.8 | 408.4 | 16.67 |
| S5 | 2.00 | 7.2 | 377.0 | 14.21 |
| S6 | 1.65 | 6.0 | 314.2 | 9.86 |
| S7 | 1.15 | 4.2 | 219.9 | 4.83 |

Tab. I: Values of some physical quantities characterizing the piston motion considered in the experiments.


[1] B. Bernu, F. Delyon, and R. Mazighi. Steady states of a column of shaken inelastic beads. *Phys. Rev. E*, 50:4551–4559, Dec 1994.

[2] Wakou Junichi, Ochiai Akinori, and Isobe Masaharu. A Langevin approach to one-dimensional granular media fluidized by vibrations. *J. Phys. Soc. Jpn.*, 77(3):1–11, 2008.

[3] Marcus V. Carneiro, Joaquim J. Barroso, and E. E N Macau. Simulation of inhomogeneous columns of beads under vertical vibration. *Math. Probl. Eng.*, 2009:345947, 2009.

[4] V. Zivkovic, M. J. Biggs, and D. H. Glass. Scaling of granular temperature in a vibrated granular bed. *Phys. Rev. E*, 83(3):1–8, 2011.

[5] Loreto Oyarte Gálvez, Nicolás Rivas, and Devaraj van der Meer. Experiments and characterization of low-frequency oscillations in a granular column. *Phys. Rev. E*, 97:042901, Apr 2018.

[6] S. Luding, E. Clément, A. Blumen, J. Rajchenbach, and J. Duran. Studies of columns of beads under external vibrations. *Phys. Rev. E*, 49:1634–1646, Feb 1994.

[7] C.S. Sandeep, K. Senetakis, D. Cheung, C.E. Choi, Y. Wang, M.R. Coop, and C.W.W. Ng. Experimental study on the coefficient of restitution of grain against block interfaces for natural and engineered materials. *Can. Geotech. J.*, 58:35, 2020.

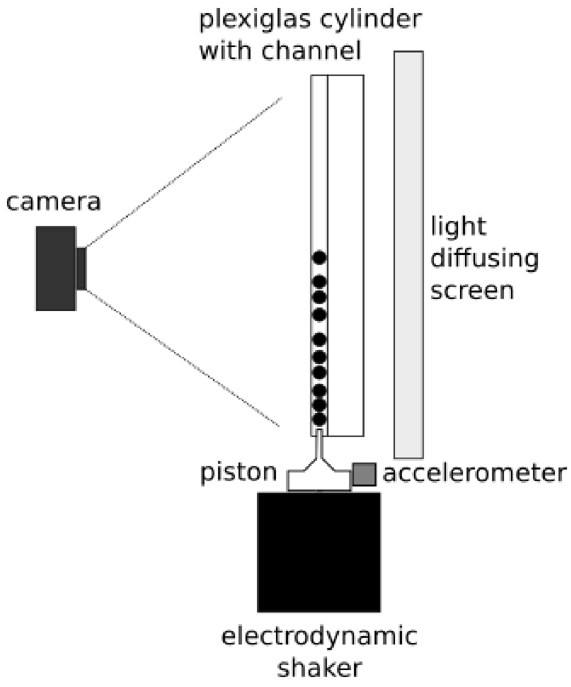


Fig S1: Scheme of the experimental setup.

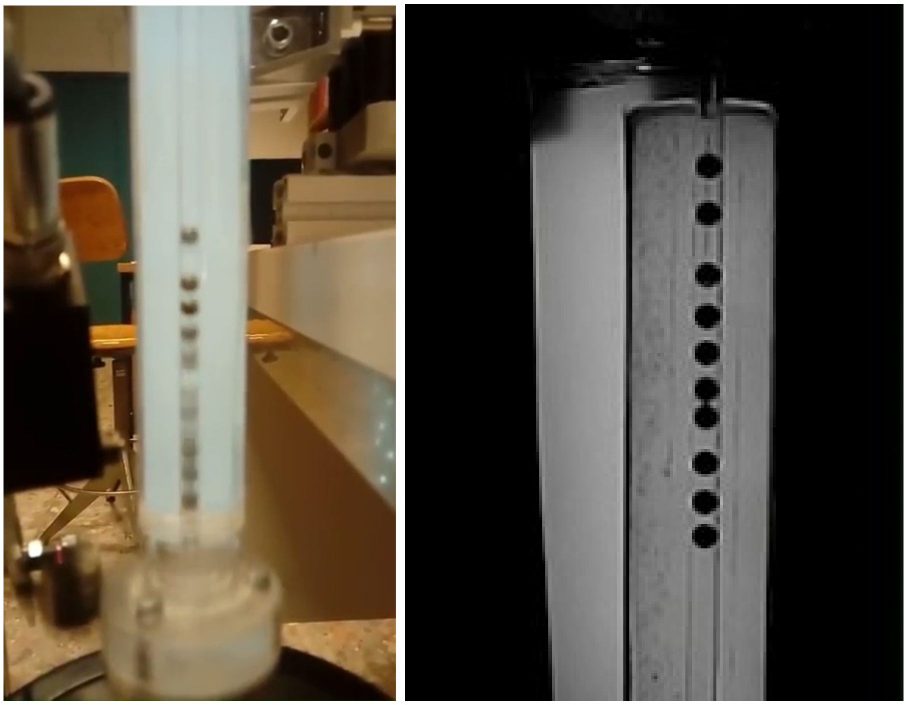

Fig. S2: Snapshot of the beads shaken within the pipe (left) and as framed by the photo camera (right).

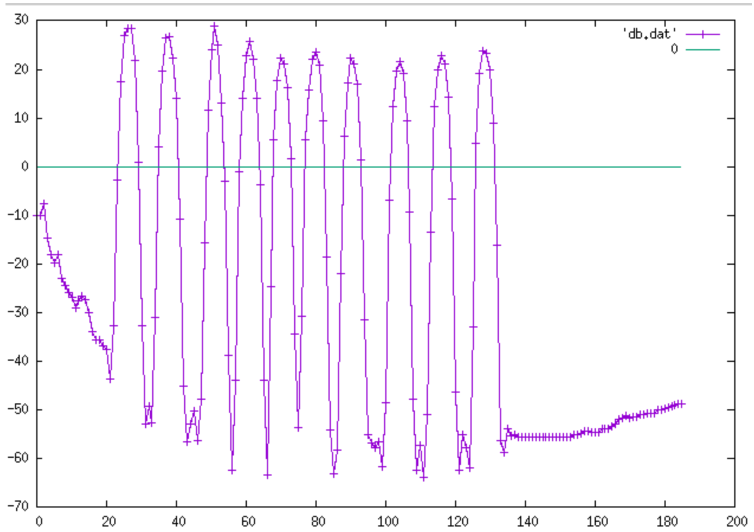


Fig. S3: Example of luminosity profile obtained after processing images. The green, horizontal, line is the threshold applied to set fitting limits around the maxima.

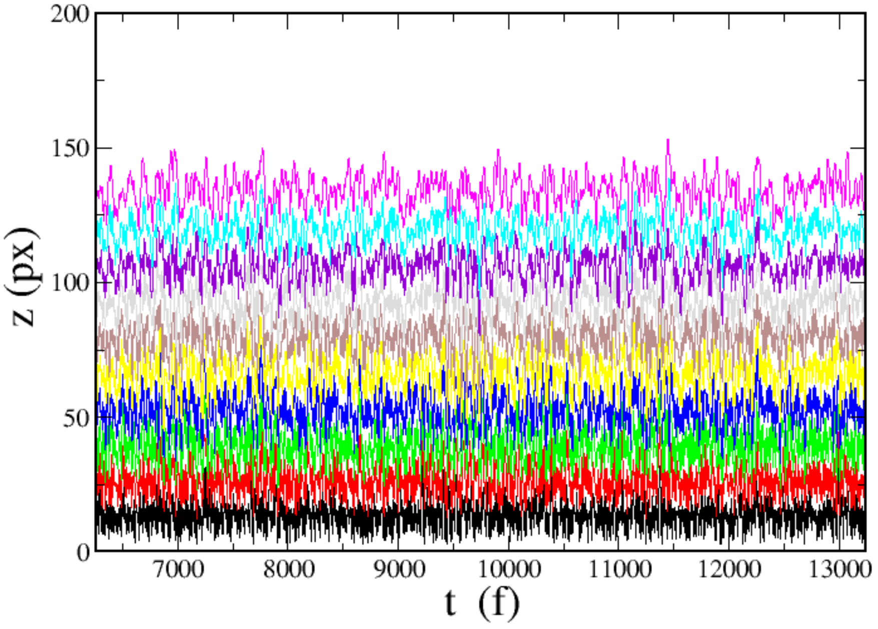


Fig. S4: Sample of the beads trajectories. Here coordinates are in pixels and time in frames.

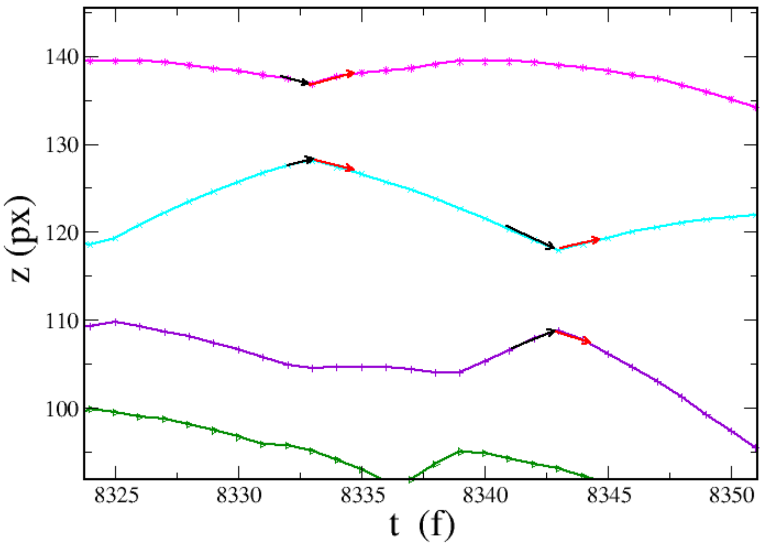


Fig. S5: Examples of collisional events employed for measuring of the restitution coefficient from Eq. (1). The arrows represent the velocity direction before (black) and after (red) collision.

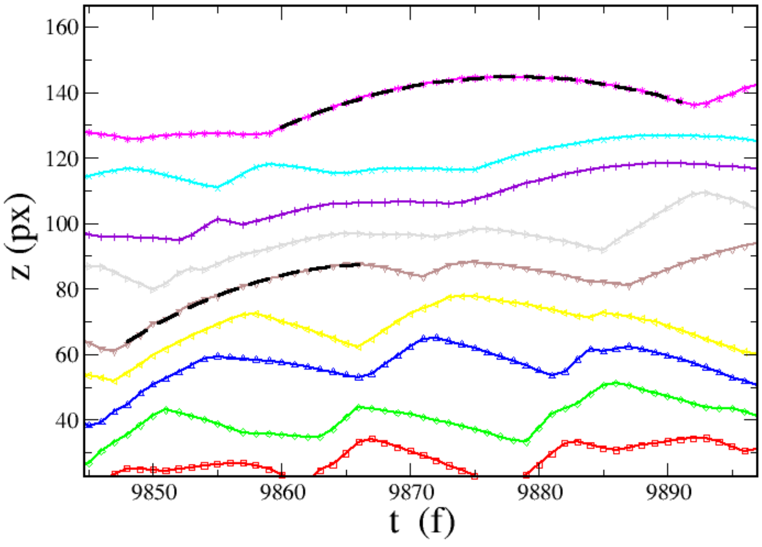


Fig. S6: Examples of fits of free trajectories with parabolic curves.
